# Supplementary material for: Tensegrity-based Robot Leg Design with Variable Stiffness
Source: arXiv:2504.19685 source file (2025-04-28)
Supplement: Supplementary file 1 [file appendix.tex]

%%%%%%%%%%%%%%%%%%%%%%%%%%%%%%%%%%%%%%%%%%%%
\onecolumn
\newpage
\appendices
\section{Mechanical Analysis of Variable Stiffness Mechanism}

\begin{table}[h!]
\centering
\caption{Symbols used for variable stiffness analysis}
\begin{tabular}{@{}llc@{}}          % Aligns content for better structure
\toprule
\textbf{Symbol}      & \textbf{Description}                                           & \textbf{Units}                          \\ \midrule
$k_s$                & Linear stiffness coefficient of the spring                    & \si{\newton\per\meter}                  \\ 
$k_c$                & Stiffness coefficient of the cable                            & \si{\newton\per\meter}                  \\ 
$k_q$                & Quadratic stiffness coefficient of the spring                 & \si{\newton\per\meter\squared}          \\ 
$x$                  & Displacement of the spring                                    & \si{\meter}                             \\ 
$x_0$                & Initial displacement of the spring due to pretension          & \si{\meter}                             \\ 
$r_p$                & Radius of the pulley                                          & \si{\meter}                             \\ 
$\theta$             & Angular displacement of the pulley                            & \si{\radian}                            \\ 
$F_0$                & Pretension force applied to the spring                        & \si{\newton}                            \\ 
$F_{\text{spring}}$  & Force exerted by the spring                                   & \si{\newton}                            \\ 
$F_{\text{cable}}$   & Force exerted by the cable                                    & \si{\newton}                            \\ 
$F_{\text{total}}$   & Total force on the pulley (spring + cable + pretension)        & \si{\newton}                            \\ 
$T_{\text{total}}$   & Total torque applied to the pulley                            & \si{\newton\meter}                      \\ 
$k_\theta$           & Rotational stiffness of the system                            & \si{\newton\meter\per\radian}           \\ \bottomrule
\end{tabular}
\end{table}

\section{Linear Springs with Pretension}

\subsection{Assumptions}
We consider the following system:
\begin{enumerate}
    \item Cable and mechanical spring are ideal linear springs.
    \item Pretension in spring and cable due to variable stiffness mechanism.
    \item Three-pointed star patella simplified as disk with ideal pulley.
    \item No loss due to friction.
    \item Static analysis: We assume that all dynamic forces have converged to equilibrium.
\end{enumerate}

\subsection{Forces and Displacements}
The displacement of the cable due to the pulley rotation is:
\begin{align}
x &= r_p \theta
\end{align}
The force in the spring due to displacement (without considering pretension) is given by Hooke's law:
\begin{align}
F_{\text{spring}} &= k_s \cdot x = k_s \cdot r_p \cdot \theta
\end{align}
The force in the cable due to its stiffness is:
\begin{align}
F_{\text{cable}} &= k_c \cdot x = k_c \cdot r_p \cdot \theta
\end{align}
The total force on each side of the pulley is the sum of the spring and cable forces plus the pretension:
\begin{align}
F_1 &= F_0 + (k_s + k_c) \cdot r_p \cdot \theta \\
F_2 &= F_0 + (k_s + k_c) \cdot r_p \cdot \theta
\end{align}

\subsection{Torque on the Pulley}
The torque on the pulley from both sides (since both springs are pulling in opposite directions) is:
\begin{align}
T_{\text{total}} &= (F_1 - F_2) \cdot r_p
\end{align}
Substituting the expressions for \( F_1 \) and \( F_2 \):
\begin{align}
T_{\text{total}} &= \left( \left(F_0 + (k_s + k_c) \cdot r_p \cdot \theta \right) - \left(F_0 + (k_s + k_c) \cdot r_p \cdot \theta \right) \right) \cdot r_p
\end{align}
Simplifying:
\begin{align}
T_{\text{total}} &= 0
\end{align}
Thus, the pretension forces cancel each other out, and only the stiffness components contribute to the torque.

\subsection{Rotational Stiffness}
The rotational stiffness $k_{\theta}$ is the rate of change of torque with respect to angular displacement:
\begin{align}
k_{\theta} &= \frac{dT_{\text{total}}}{d\theta}
\end{align}
From the spring and cable forces:
\begin{align}
T_{\text{springs}} &= (k_s + k_c) \cdot r_p^2 \cdot \theta
\end{align}
Thus, the rotational stiffness is:
\begin{align}
k_{\theta} &= (k_s + k_c) \cdot r_p^2
\end{align}

\subsection{Conclusion}
The rotational stiffness of the pulley system is:
\begin{align}
k_{\theta} = (k_s + k_c) \cdot r_p^2
\end{align}
It depends on the spring stiffness, the cable stiffness, and the pulley radius, but is independent of the pretension $F_0$, as the pretension forces cancel each other out.

\section{Multi-Spring System: Series and Parallel Configurations}
Now we examine the influence of a multi-spring system in two configurations: one where the springs are in series, and one where the springs are in parallel.

\subsection{Series Configuration}
In a series configuration, two springs with stiffnesses $k_{s1}$ and $k_{s2}$ are connected in series. The total stiffness $k_{\text{series}}$ is given by the reciprocal of the sum of the reciprocals of the individual stiffnesses:
\begin{align}
\frac{1}{k_{\text{series}}} &= \frac{1}{k_{s1}} + \frac{1}{k_{s2}} \\
k_{\text{series}} &= \frac{k_{s1} \cdot k_{s2}}{k_{s1} + k_{s2}}
\end{align}
In this configuration, the total stiffness decreases as the springs are combined, resulting in a \textbf{lower rotational stiffness} $k_\theta$ compared to a single spring with stiffness $k_s$.

Thus, the rotational stiffness in the series configuration is:
\begin{align}
k_\theta^{\text{series}} &= \left( \frac{k_{s1} \cdot k_{s2}}{k_{s1} + k_{s2}} + k_c \right) \cdot r_p^2
\end{align}
The system becomes more compliant (less stiff) as more springs are added in series.

\subsection{Parallel Configuration}
In a parallel configuration, the total stiffness $k_{\text{parallel}}$ is the sum of the individual spring stiffnesses:
\begin{align}
k_{\text{parallel}} &= k_{s1} + k_{s2}
\end{align}
In this case, the total stiffness increases as more springs are added in parallel, leading to a higher rotational stiffness $k_\theta$.

Thus, the rotational stiffness in the parallel configuration is:
\begin{align}
k_\theta^{\text{parallel}} &= \left( k_{s1} + k_{s2} + k_c \right) \cdot r_p^2
\end{align}
This configuration results in a stiffer system, as the effective stiffness increases with the number of springs in parallel.

\subsection{Influence of Pretension in Multi-Spring Systems}
It is important to note that in both the series and parallel configurations, the \textbf{pretension} forces $F_0$ do not affect the rotational stiffness $k_\theta$. Pretension introduces a constant force, but it does not influence the rate of change of torque with respect to angular displacement, which defines the rotational stiffness.

In both the series and parallel configurations, the total torque is influenced only by the spring stiffnesses and cable stiffness. The pretension term cancels out, as shown in the previous sections, and does not appear in the final expression for $k_\theta$. Therefore, regardless of the spring configuration, the rotational stiffness remains \textbf{independent of pretension}.

\subsection{Conclusion on Multi-Spring Configurations}
In a multi-spring system:
\begin{itemize}
    \item In the \textbf{series configuration}, the total stiffness decreases, leading to a lower $k_\theta$, which makes the system more compliant.
    \item In the \textbf{parallel configuration}, the total stiffness increases, resulting in a higher $k_\theta$, making the system stiffer.
    \item In both configurations, the \textbf{pretension} $F_0$ does not influence the rotational stiffness $k_\theta$, as it introduces a constant force that cancels out when calculating the rate of change of torque with respect to angular displacement.
\end{itemize}

\section{Quadratic Springs with Pretension}
Now we extend the analysis to a system where the spring has a quadratic stiffness, and we account for pretension.

\subsection{Quadratic and Linear Stiffness Model}
For a spring with both linear and quadratic stiffness, the force exerted by the spring is given by:
\begin{align}
F_{\text{spring}} &= k_l \cdot x + k_q \cdot x^2
\end{align}
where $k_l$ is the linear stiffness coefficient, $k_q$ is the quadratic stiffness coefficient, and $x = r_p \cdot \theta$ is the displacement due to angular motion of the pulley.

If pretension $F_0$ is applied, causing an initial displacement $x_0$, the total force becomes:
\begin{align}
F_{\text{spring}} &= k_l \cdot (x + x_0) + k_q \cdot (x + x_0)^2
\end{align}
The pretension force is related to the initial displacement by:
\begin{align}
F_0 &= k_l \cdot x_0 + k_q \cdot x_0^2
\end{align}

\subsection{Total Force and Torque with Linear and Quadratic Terms}
The total force, accounting for both pretension and angular displacement, is:
\begin{align}
F_{\text{total}} &= k_l \cdot \left( x_0 + r_p \cdot \theta \right) + k_q \cdot \left( x_0 + r_p \cdot \theta \right)^2
\end{align}
Expanding the square term:
\begin{align}
F_{\text{total}} &= k_l \cdot \left( x_0 + r_p \cdot \theta \right) + k_q \cdot \left( x_0^2 + 2 \cdot x_0 \cdot r_p \cdot \theta + (r_p \cdot \theta)^2 \right) \\
F_{\text{total}} &= k_l \cdot x_0 + k_l \cdot r_p \cdot \theta + k_q \cdot x_0^2 + 2 \cdot k_q \cdot x_0 \cdot r_p \cdot \theta + k_q \cdot (r_p \cdot \theta)^2
\end{align}
Simplifying the expression:
\begin{align}
F_{\text{total}} &= F_0 + (k_l + 2 \cdot k_q \cdot x_0) \cdot r_p \cdot \theta + k_q \cdot r_p^2 \cdot \theta^2
\end{align}

The corresponding torque generated by the spring force is:
\begin{align}
T_{\text{total}} &= F_{\text{total}} \cdot r_p \\
T_{\text{total}} &= F_0 \cdot r_p + (k_l + 2 \cdot k_q \cdot x_0) \cdot r_p^2 \cdot \theta + k_q \cdot r_p^3 \cdot \theta^2
\end{align}

\subsection{Rotational Stiffness with Linear and Quadratic Terms}
The rotational stiffness $k_\theta$ is the derivative of the total torque with respect to $\theta$:
\begin{align}
k_\theta &= \frac{dT_{\text{total}}}{d\theta} \\
k_\theta &= (k_l + 2 \cdot k_q \cdot x_0) \cdot r_p^2 + 2 \cdot k_q \cdot r_p^3 \cdot \theta
\end{align}

Substituting $x_0$ from the equation for pretension:
\begin{align}
x_0 &= \frac{-k_l \pm \sqrt{k_l^2 + 4 k_q F_0}}{2k_q}
\end{align}

\subsection{Conclusion for Combined Linear and Quadratic Springs}
In a system with both linear and quadratic springs:
\begin{itemize}
    \item The rotational stiffness $k_\theta$ includes both linear and quadratic terms and is influenced by both the pretension $F_0$ and the angular displacement $\theta$.
    \item Pretension $F_0$ modifies both the linear and quadratic terms, affecting the baseline stiffness.
    \item The stiffness grows with angular displacement due to the quadratic term $2 \cdot k_q \cdot r_p^3 \cdot \theta$, making the system progressively stiffer as the pulley rotates.
\end{itemize}
This model captures the combined effects of linear and non-linear stiffness and accounts for the influence of pretension on the system's behavior. The rotational stiffness is non-linear in the case of quadratic springs, and pretension adds to the stiffness baseline, making the system more resistant to rotation.

\section{Comparison of different Spring Configurations}

\begin{figure}[H]
    \centering
    \subfloat[linear spring]{%
    \includegraphics[height=6.0cm]{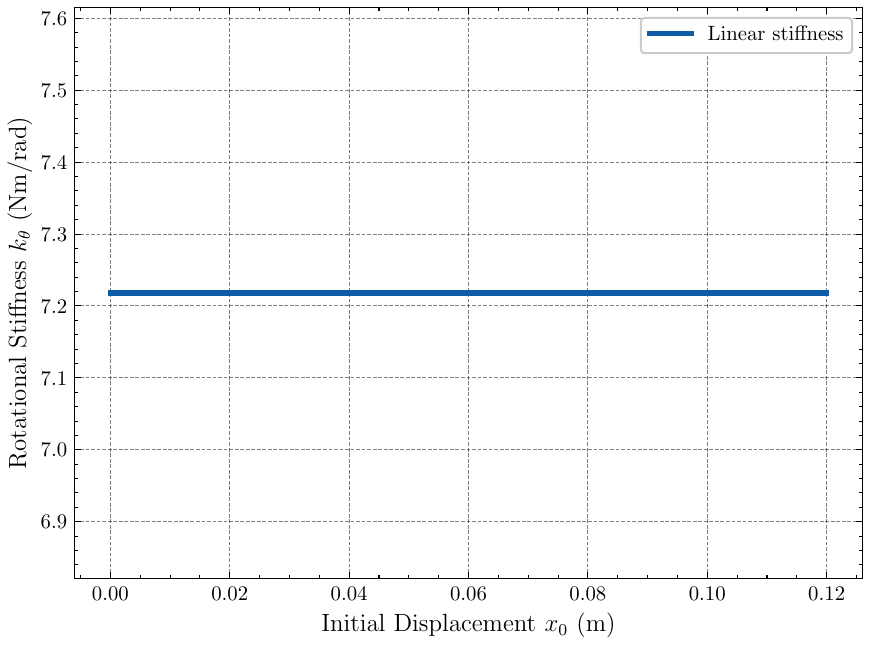} 
    }
    \hfill
    \subfloat[quadratic spring]{%
    \includegraphics[height=6.0cm]{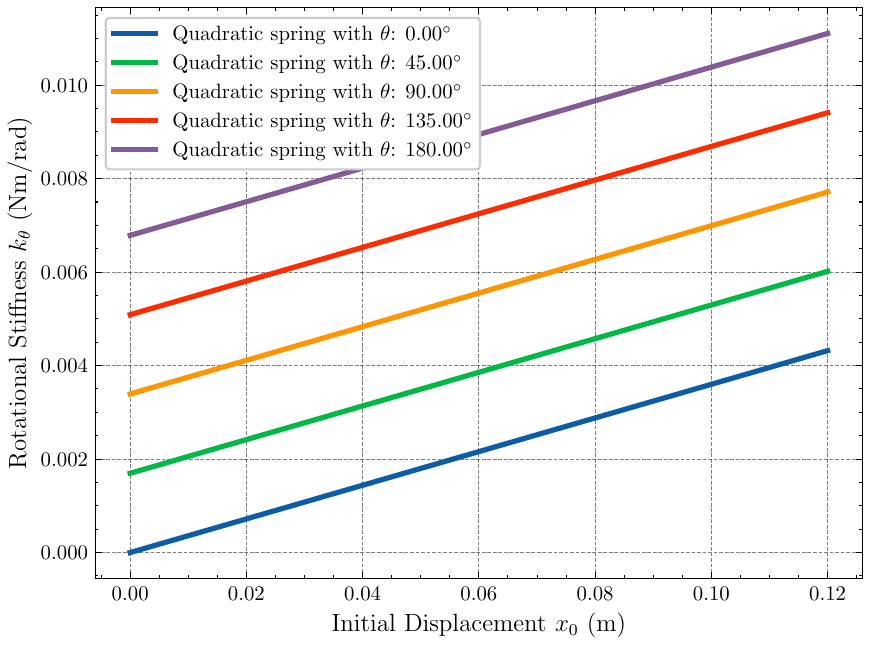}
    }
    \caption{Rotational stiffness for (a) linear springs, (b) quadratic springs.}
\end{figure}

\section{Lead screw Dimensioning}

A lead screw mechanism can be used to adjust the pre-tension of a spring by translating rotational motion into linear displacement. The adjustment of the spring's initial displacement, denoted as $x_0$, modifies the pre-tension force applied to the system. The dimensioning follows the methodology described by Budynas et al. \cite{budynas2011shigley}.

\begin{table}[h!]
\centering
\caption{Symbols, Descriptions, and Units for Lead Screw Design}
\setlength{\tabcolsep}{10pt} % Adjusts column spacing
\begin{tabular}{@{}llc@{}}
\toprule
\textbf{Symbol} & \textbf{Description} & \textbf{Units} \\ \midrule
$k_s$           & Spring stiffness & \si{\newton\per\meter} \\
$x_0$           & Initial displacement (pre-tension) & \si{\meter} \\
$F_{\text{axial}}$ & Axial force at displacement $x_0$ & \si{\newton} \\
$L$             & Lead of the screw & \si{\meter\per\text{rev}} \\
$D_m$           & Mean diameter of the screw & \si{\meter} \\
$f$             & Coefficient of friction & dimensionless \\
$\lambda$       & Lead angle & \si{\degree} \\
$T_{\text{req}}$ & Required torque to move the nut & \si{\newton\meter} \\
\bottomrule
\end{tabular}
\end{table}

\subsection*{Torque Required to Adjust Pre-Tension}
We assume that forces applying to the variable stiffness mechanism dominantly rely on the pre-tensioning of the strings due to the variable stiffness mechanism itself. It assumed due to payload and other external forces only shift forces within the antagonistic configuration, negligibly affecting the overall applying forces.

We consider the following system:
\begin{itemize}
    \item Spring stiffness: $ k_s = 500 \, \si{\newton\per\meter} $
    \item Desired initial displacement: $ x_0 = 0.071 \, \si{\meter} $
    \item Mean diameter of the screw: $ D_m = \SI{8}{\milli\meter} $
    \item Lead of the screw: $ L = \SI{4}{\milli\meter} $
    \item Coefficient of friction: $ \mu_r = 0.15$ (see Shigley table for steel-bronze without lubrication \cite{budynas2011shigley}).
\end{itemize}

\subsection*{Step 1: Calculate the Axial Force}

The axial force $ F_{\text{axial}} $ depends mainly on the pre-tension forces of the springs. We assume the maximum load case of two joints, each consisting of two parallel-slack springs in an antagonistic configuration, applying forces on one lead screw with maximum pre-tension.
\begin{align}
F_{\text{axial}} &=  4 \cdot F_{spring} \nonumber \\
F_{\text{axial}} &= \SI{320}{\newton}
\end{align}

\subsection*{Step 2: Calculate the Lead Angle}

The lead angle is calculated as:
\begin{align}
\lambda &= \tan^{-1} \left( \frac{L}{\pi D_m} \right) \nonumber \\
\lambda &\approx \SI{0.158}{\radian} \approx 9.04^\circ
\end{align}

\subsection*{Step 3: Calculate the Required Torque}

The torque required to overcome friction and move the nut is calculated using Shigley's formula:
\begin{align}
T_{\text{req,raise}} &= \frac{F_{\text{axial}} \cdot D_m}{2} \cdot \left( \frac{L + \pi \mu_r D_m}{\pi D_m - \mu_r L} \right) \\
T_{\text{req,raise}} &\approx \SI{0.2027}{\newton\meter}
\end{align}

\begin{align}
T_{\text{req,lower}} &= \frac{F_{\text{axial}} \cdot D_m}{2} \cdot \left( \frac{L - \pi \mu_r D_m}{\pi D_m + \mu_r L} \right) \\
T_{\text{req,lower}} &\approx \SI{0.0057}{\newton\meter}
\end{align}

Thus, the required torque to achieve a displacement of \SI{10}{\milli\meter} is approximately \SI{0.2027}{\newton\meter}. We selected the small form factor, commercially available and low-cost stepper motor PG25L-D24-HHC1 by manufacturer Minebea-Mitsumi. According to the manufacturer, it provides a torque of up to $T = \SI{0.45}{\newton\meter}$, sufficing the computed required torque.

\subsection*{Self-Locking Condition}
A lead screw can be self-locking if the coefficient of friction $ \mu_r $ exceeds the tangent of the lead angle $ \lambda $. The condition for self-locking is:
\begin{align}
\mu_r > \tan(\lambda)
\end{align}
For this example:
\begin{align}
\mu_r &= 0.15, \nonumber \\
\tan(\lambda) &= 0.1592
\end{align}

Since $ \mu_r > \tan(\lambda) $, the screw is self-locking, meaning it will not back-drive under load. Under full load, the proposed variable stiffness mechanism is not self-locking and requires holding torque of the screw drive mechanism.

\section{Variable Stiffness Mechanism}

For the variable stiffness mechanism, the systems require nonlinear spring behavior. To create quadratic spring stiffness, we use 3 springs in a parallel configuration in series with different length cables.  

\begin{figure}[H]
    \centering
    \subfloat[Experimental setup]{%
    \includegraphics[height=8.0cm]{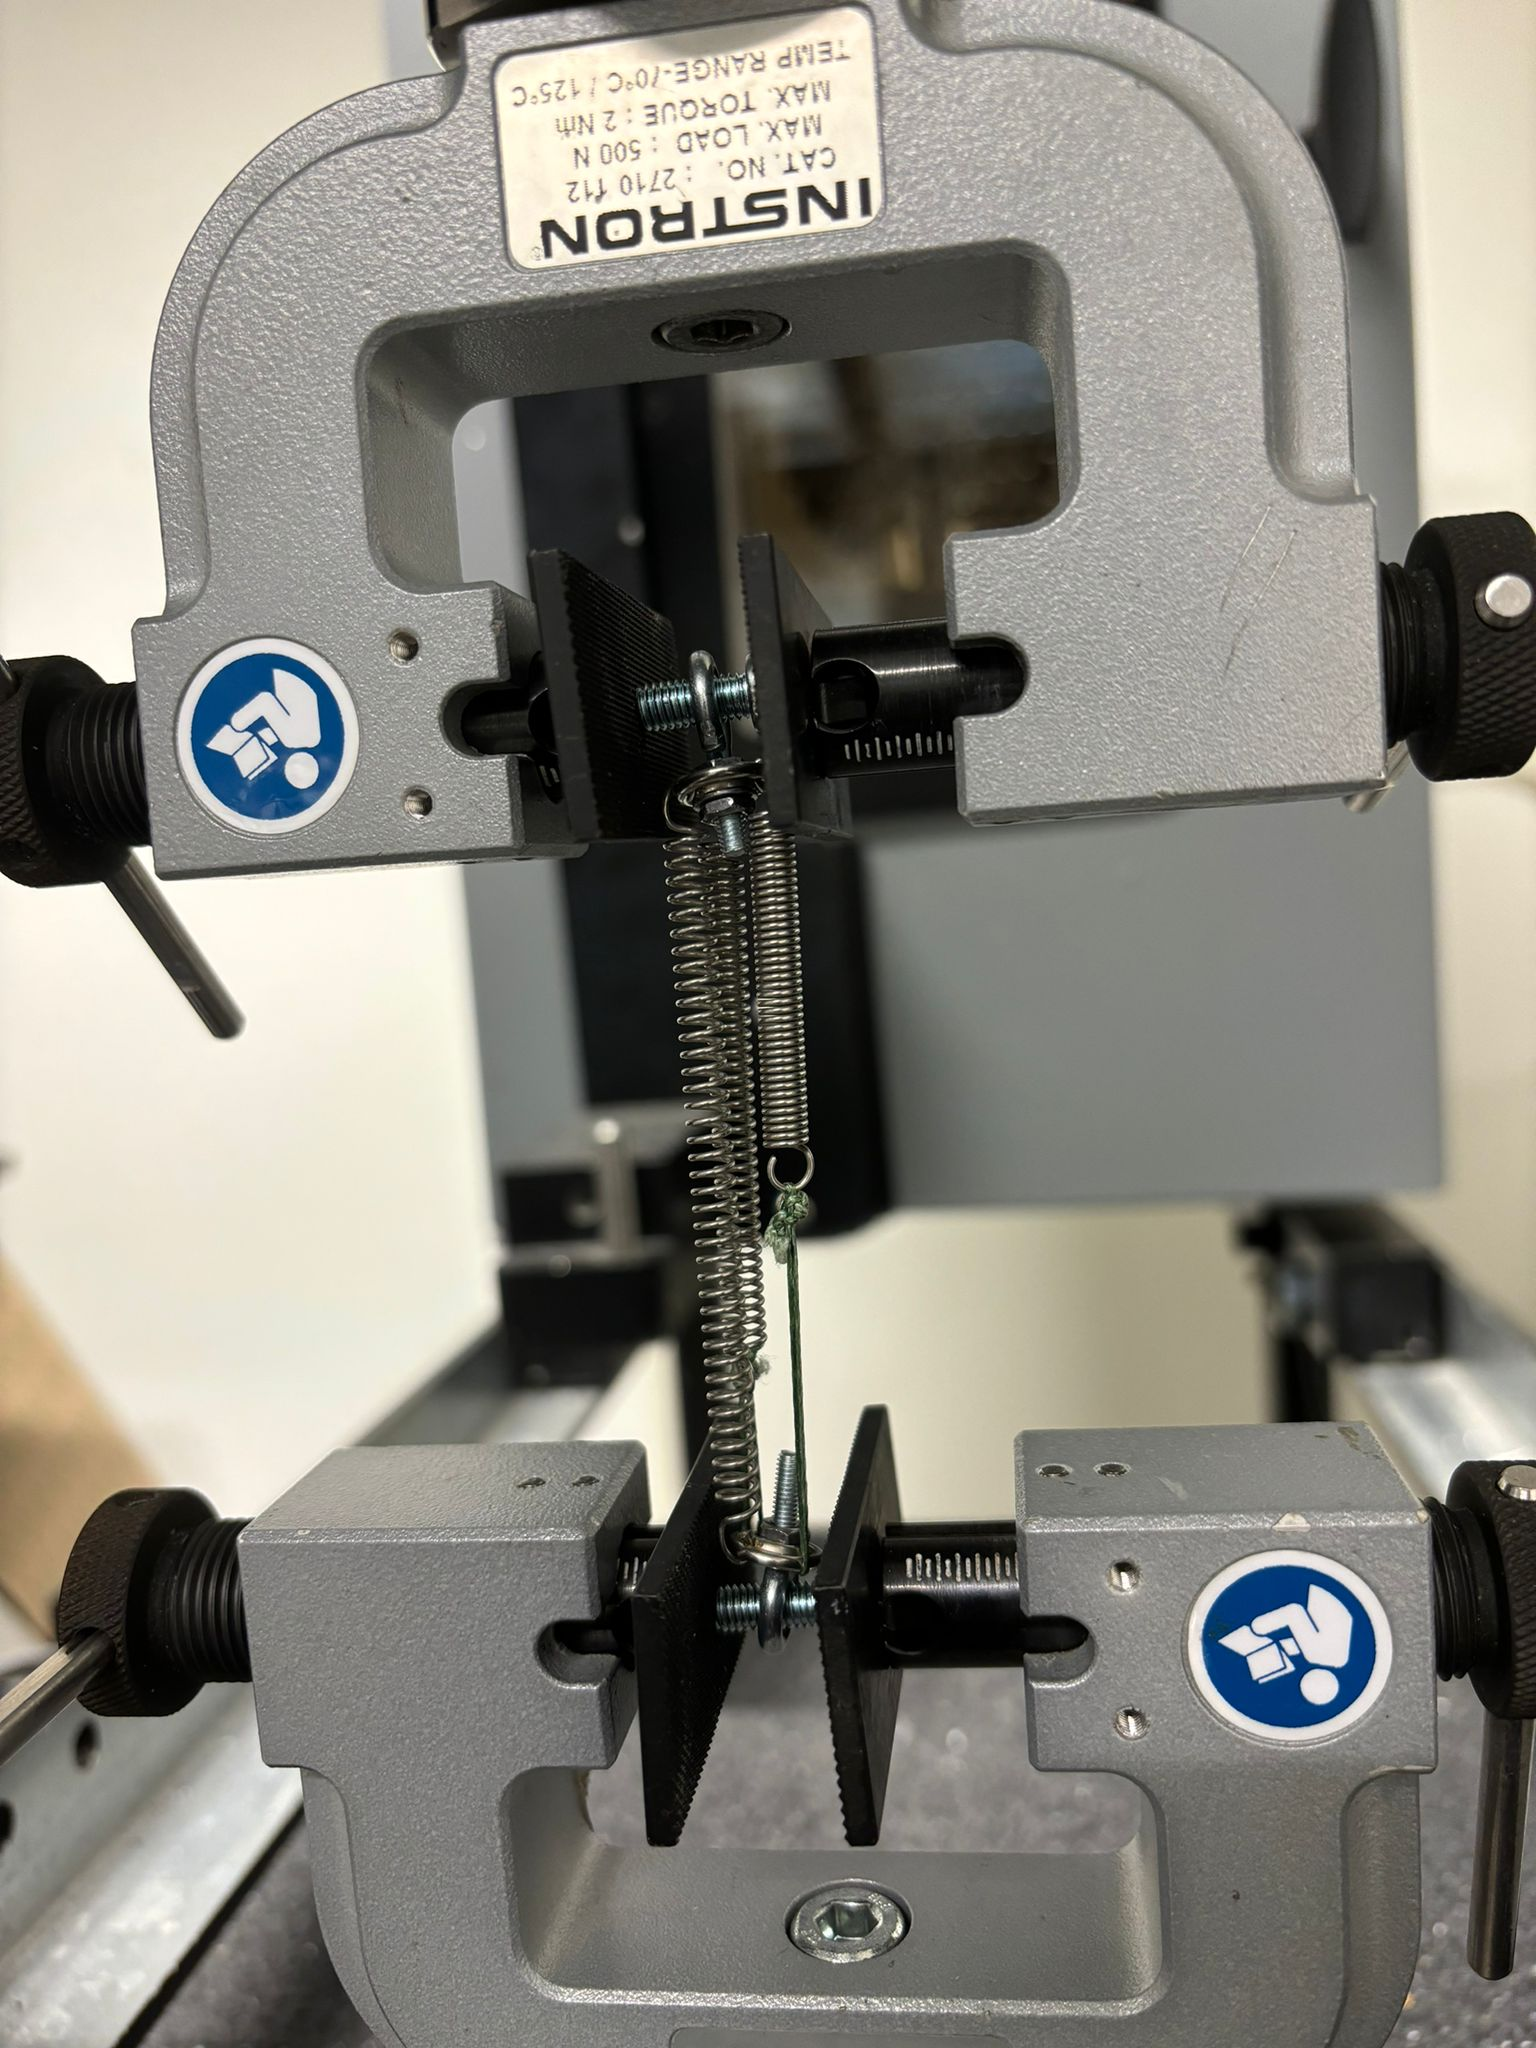} 
    }
    \hspace{0.5cm}
    \subfloat[Measurement]{%
    \includegraphics[height=8.0cm]{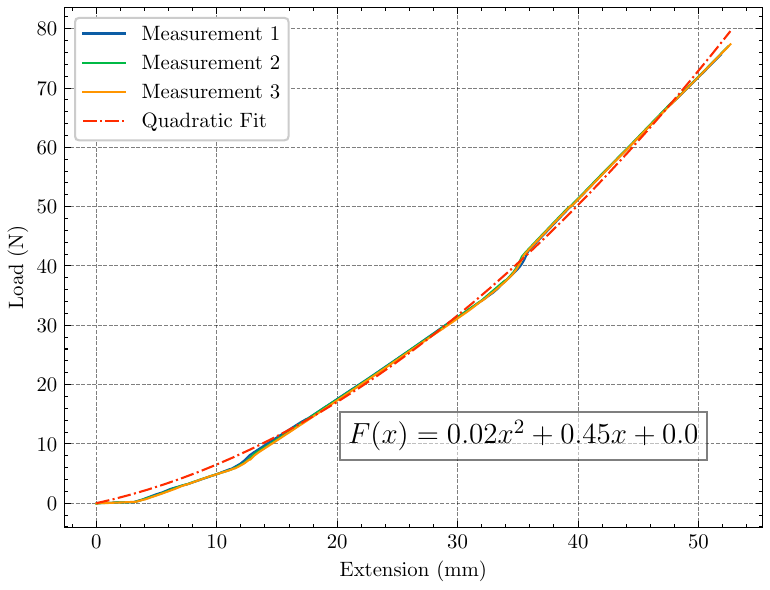}
    }
    \caption{Load-extension measurement of parallel-slack springs, closely resembling quadratic spring behavior.}
\end{figure}

The cables consist out of highly durable polyester-nylon paracord with a diameter of \SI{1.18}{\milli\meter} from the manufacturer Atwood Rope MFG. The cables show low elasticity, resulting in negligible stiffness for the parallel-slack spring mechanism.

We perform simple extension-load experiments to determine the stiffness behavior of the spring configuration. In the extension range of \SI{0}{\milli\meter} to \SI{50}{\milli\meter}, the mechanism closely resembles quadratic behavior. We use least-squares to fit an unbiased quadratic function $F(x)=ax^2+bx$. The coefficients $a=0.02$ and $b=0.45$ provide a nearly perfect fit with a $R^2 = 0.9983$.

\section{Joint characterization}
%\subsection{Tensegrity joint characterization}

%In order to test some passive properties of the Y-Y-Y joint and see the effect that the dimensioning of the tendons have on them, the two following experiments have been realized. The passive properties of the joint are the properties that the joint has before the actuation and variable compliance mechanism have been introduced. The tested parameters are the resistance to compression, which defines how much the joint deforms under coaxial loading, and the passive resistance to rotation, which defines the torque required to rotate the joint without any charge or actuation (the elastic tendons need to deform slightly to allow joint rotation).

In order to characterize some mechanical properties of the tensegrity joint and to determinate an appropriate dimensioning for its TPU tendons, two additional experiments were realized. These experiments aim to characterize the joint's passive resistance to rotation and its passive resistance to coaxial compression. The term “passive” indicates that the joint is not connected to any actuation cables, meaning that the measured resistance is only due to the deformation of the tendons. Four different sets of tendons will be tested in these experiments. Each set is defined by the tendons' cross-sectional area ($8mm^2$ and $12mm^2$) and three levels of pre-tension (70\%, 80\% and 90\% with reference to the length of the tendons on the tensegrity structure). The 70\% $12mm^2$ and 90\% $8mm^2$ variants were not tested, as they were respectively too tight and too loose. The set of tendons minimizing joint resistance to rotation and maximizing resistance to coaxial loading will be used for the rest of the experiments.

\subsection{Passive joint resistance to rotation}

\begin{figure}[!h]
\centering
\subfloat[Photo taken during the test]
{\label{fig:test_passive_rotation}
\includegraphics[width=.30\columnwidth]{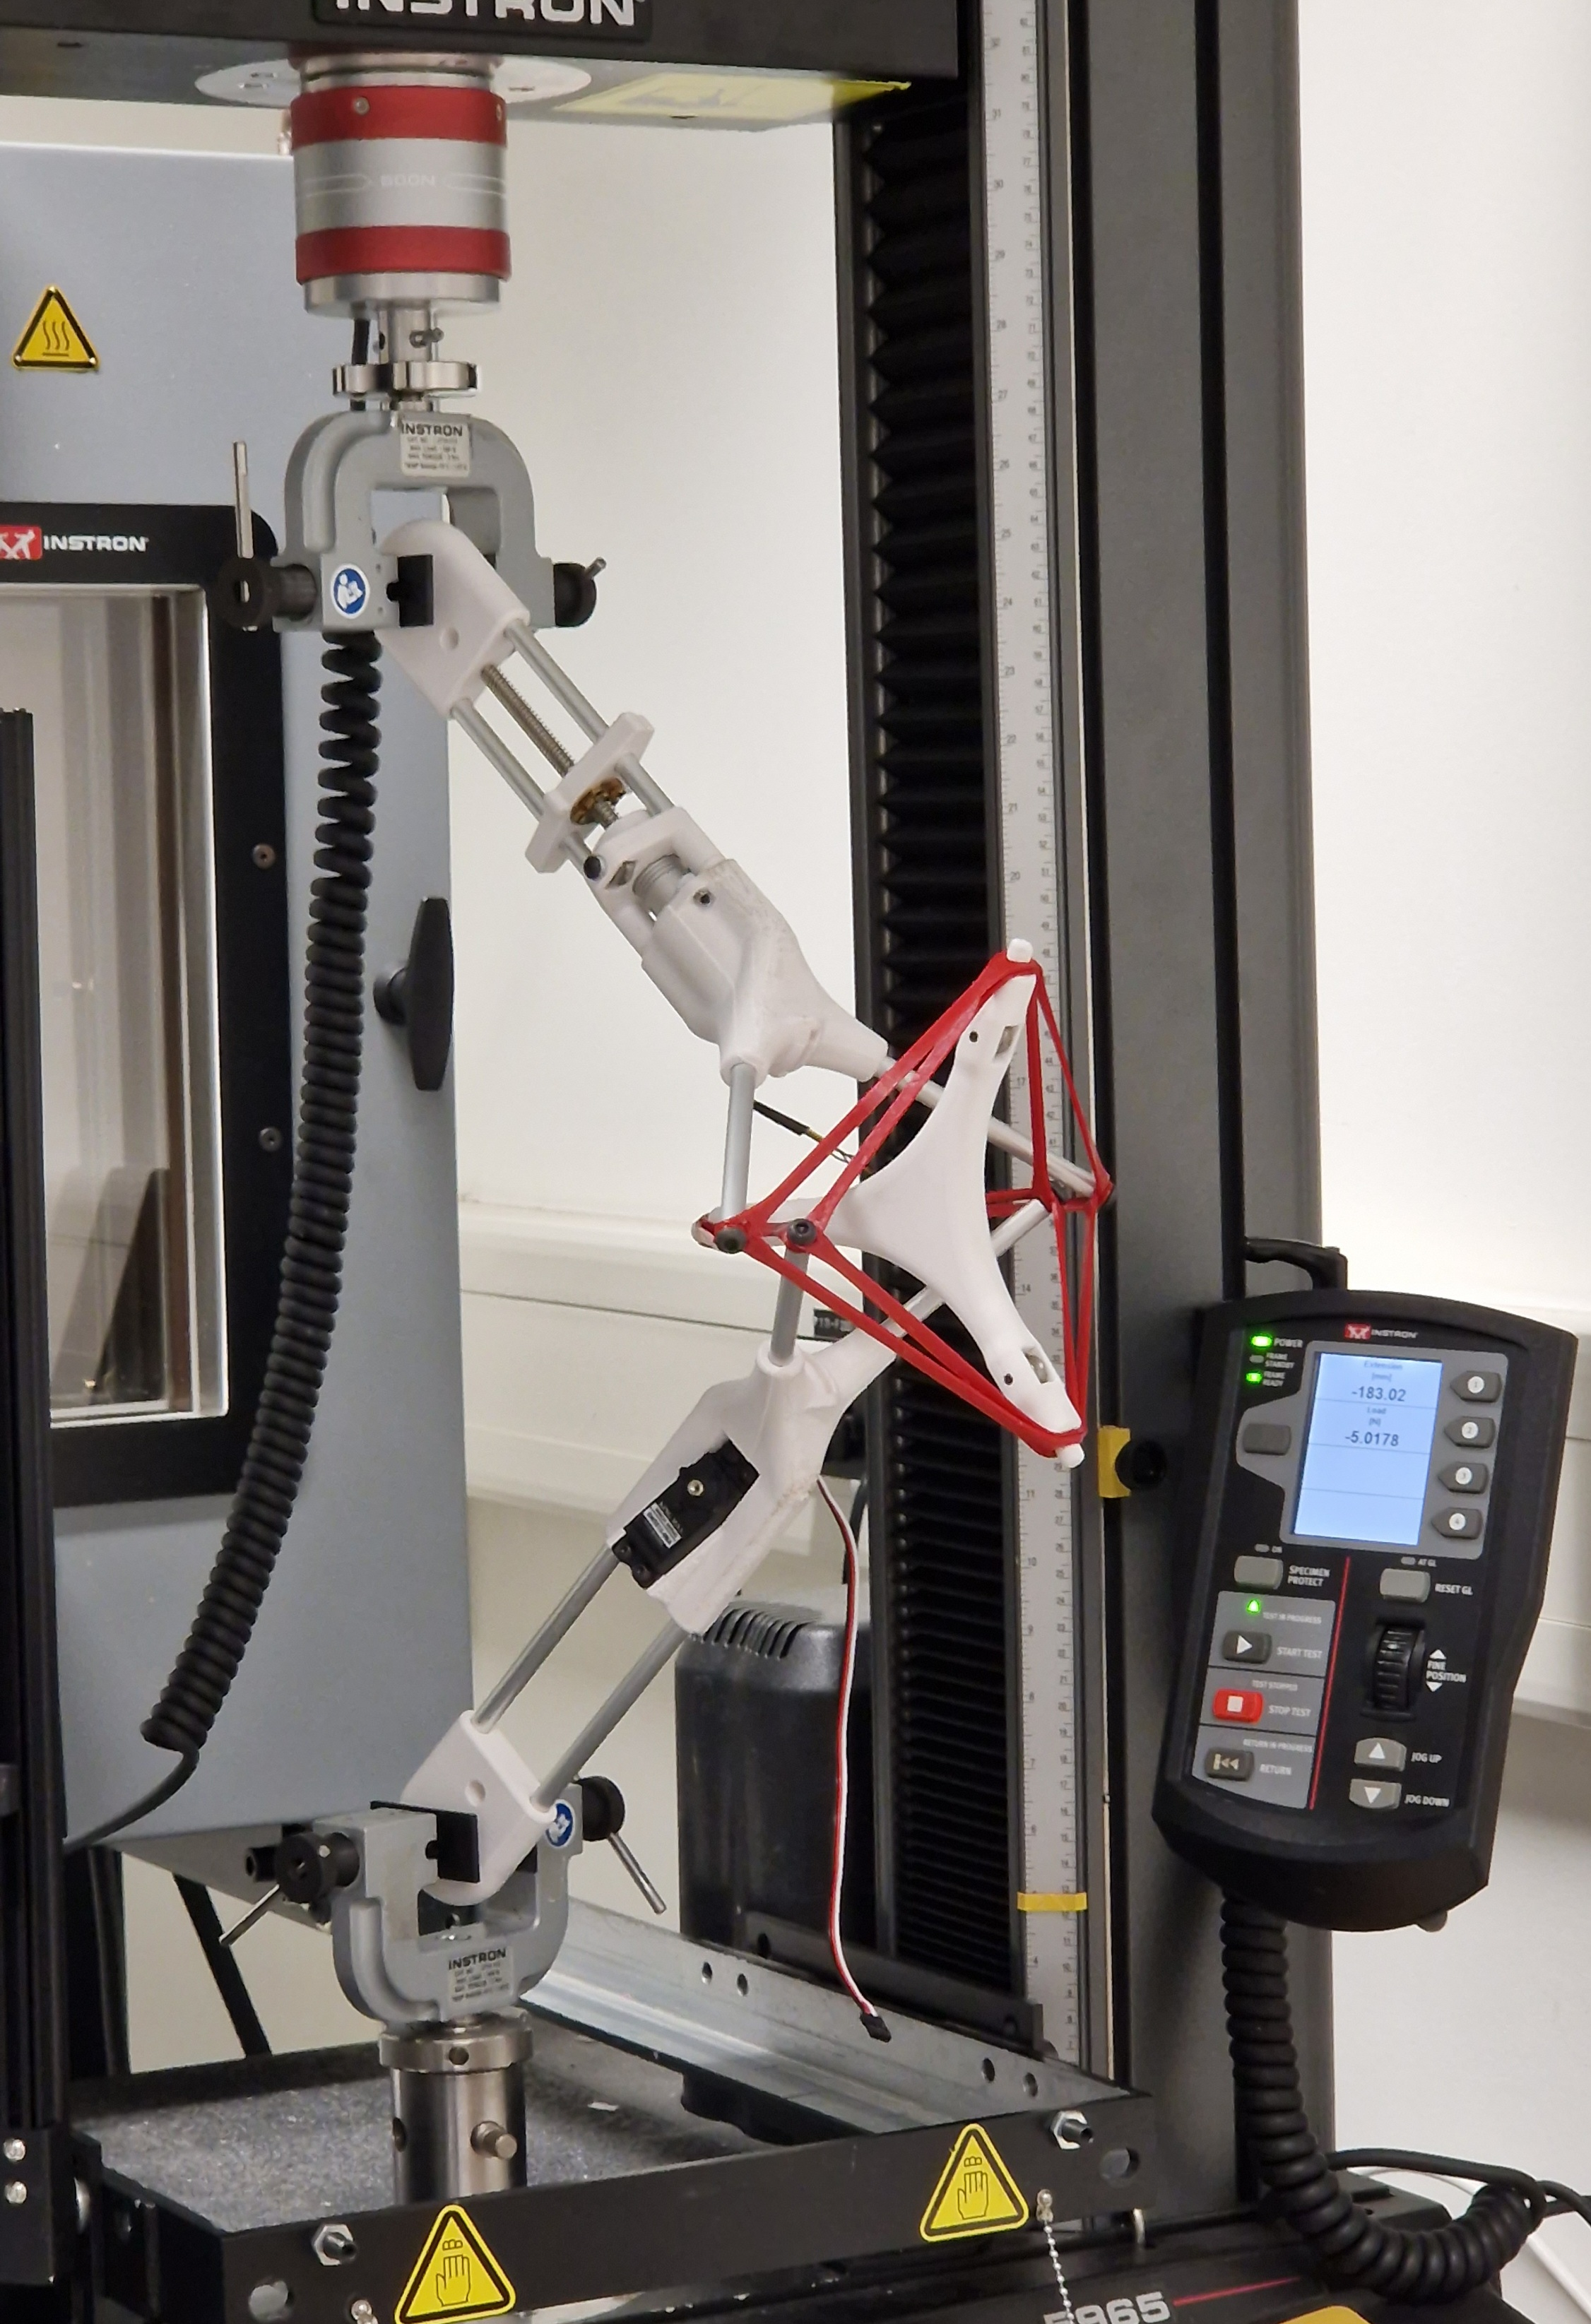}} \quad
\subfloat[Schema representing the test]
{\label{fig:test_joint_schema_passive}%
\includegraphics[width=.30\columnwidth]{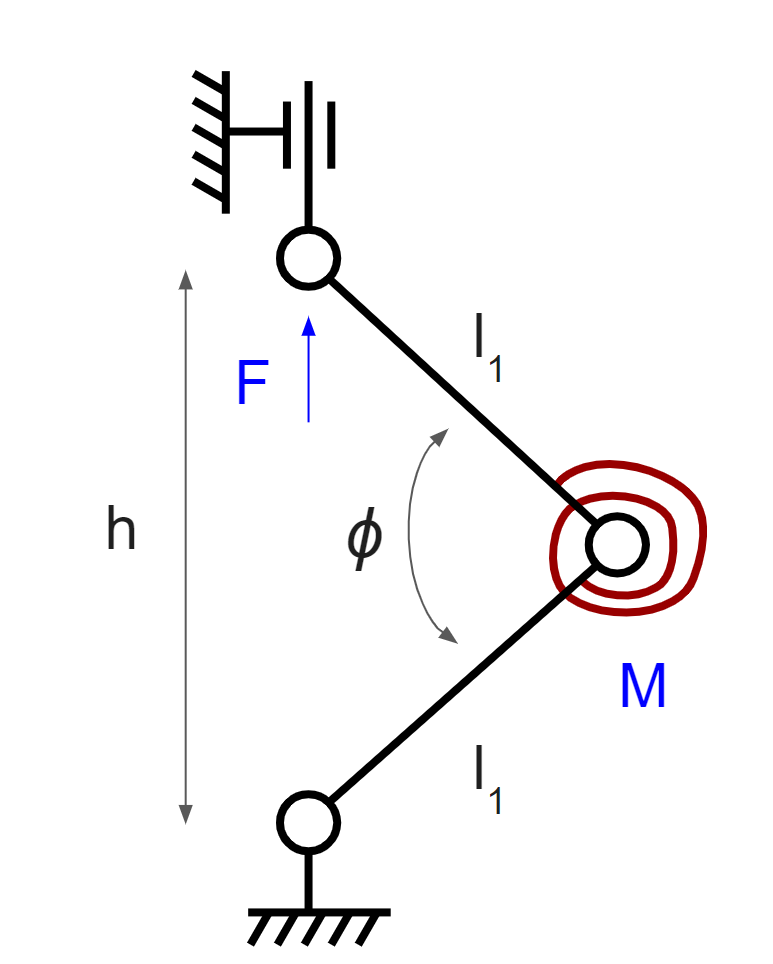}} \quad
\caption{Photo (a) and schema (b) of the test realized on the joint to measure its passive resistance to rotation when not actuated}
\label{fig:test_passive_rotation}
\end{figure}

In this experiment, each extremity of the joint is connected to an arm of total length $l_1 = 310mm$ which is then itself connected, free to rotate, to one of the extremities of a tensile test machine, as described in the schema \ref{fig:test_joint_schema_passive}. The joint is thus allowed to rotate depending on the distance between the two extremities, h. The relation between the joint angle $\phi$ and the value of h is given by the following equation:
\begin{equation}
\phi = 2 arcsin\left (\frac{h}{2 l_1}  \right )
\label{eq:phi}
\end{equation}
The joint angle is originally set to $\phi = 120°$ as it is the equilibrium position of the joint. It is then forced to bend until it reaches its minimum angle of 10° (performed by decreasing the value of h at the speed of $4mm/s$). The reaction force F is measured by the machine. It is originally set to $0N$ in order to subtract the effects of gravity on the measurements. As the joint can, in this case, be approximated as a rotational spring, the torque compensated by this spring can be calculated from the following formula:

\begin{equation}
M = F l_1 cos\left (\frac{\phi}{2}  \right )
\label{eq:torque}
\end{equation}

The results of this experiment are presented on Figure: \ref{fig:test_passive_resistance}.

\begin{figure}[!h]
\centering 
\includegraphics[width=.8\columnwidth]{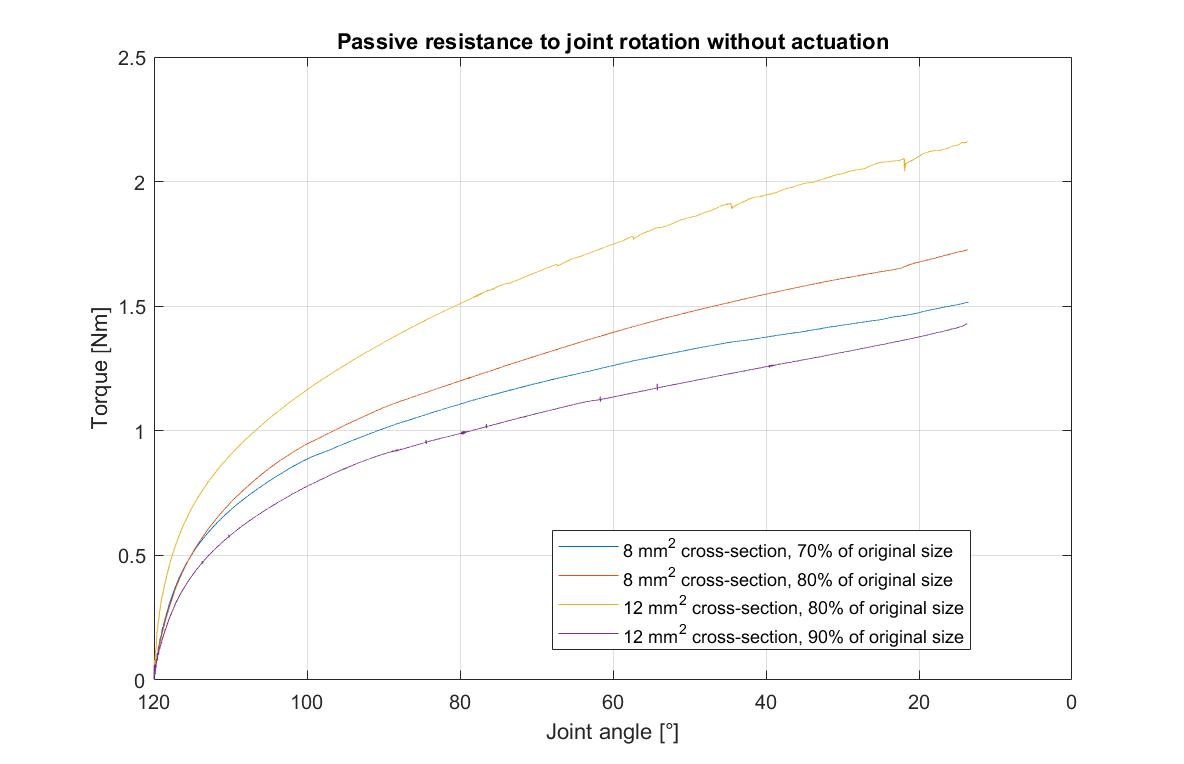} 
\caption{Plot of the measured passive resistance to rotation of the joint without actuation and for different sizing of tendons}
\label{fig:test_passive_resistance} 
\end{figure}

This graph shows that the join opposes some resistance to rotation due to the elastic deformation of its tendons, increasing logarithmically as the joint rotates away from its equilibrium point (120°). It also suggests that increasing both pre-tension and cross-sectional area increase the joint's passive resistance to rotation. %Additionally, as the cross-sectional area grows, the effect of higher pre-tension on passive resistance becomes more significant. Finally, for a given level of pre-tension, tendons with larger cross-sectional areas provide greater resistance to joint rotation.

%It is noticeable on this graph that both an increase in pre-tension and in cross-section area lead to an increase in the joint's passive resistance to rotation. It is also observable that as the cross-sectional area increases, the impact of elevating the degree of pretension on passive resistance to rotation becomes more pronounced. Finally, for the same level of pre-tension, the set of tendons with a larger cross-section induces more resistance to joint rotation. 
%This is due to the fact that the tension in the tendons follows Hook's law (see: \ref{equ:Hook}) and thus an increase in the cross-section area will induce an increase in the force developed by the elastic.

%In the context of legged robotics, a rotational joint is generally assumed to offer the least possible resistance to rotation. The set of tendons with a cross-section of $12mm^2$ and the lengths defined by a degree of pre-tension of 90\% on Table: \ref{tab:pretension}. A possible exception would be if the robot needs to remain stable at a certain position when not actuated (turned off) but this feature will not be considered in this report. 

\subsection{Passive joint resistance to coaxial loading}

\begin{figure}[!h]
\centering
\subfloat[Photo taken during the test]
{\label{fig:test_compression}
\includegraphics[width=.35\columnwidth]{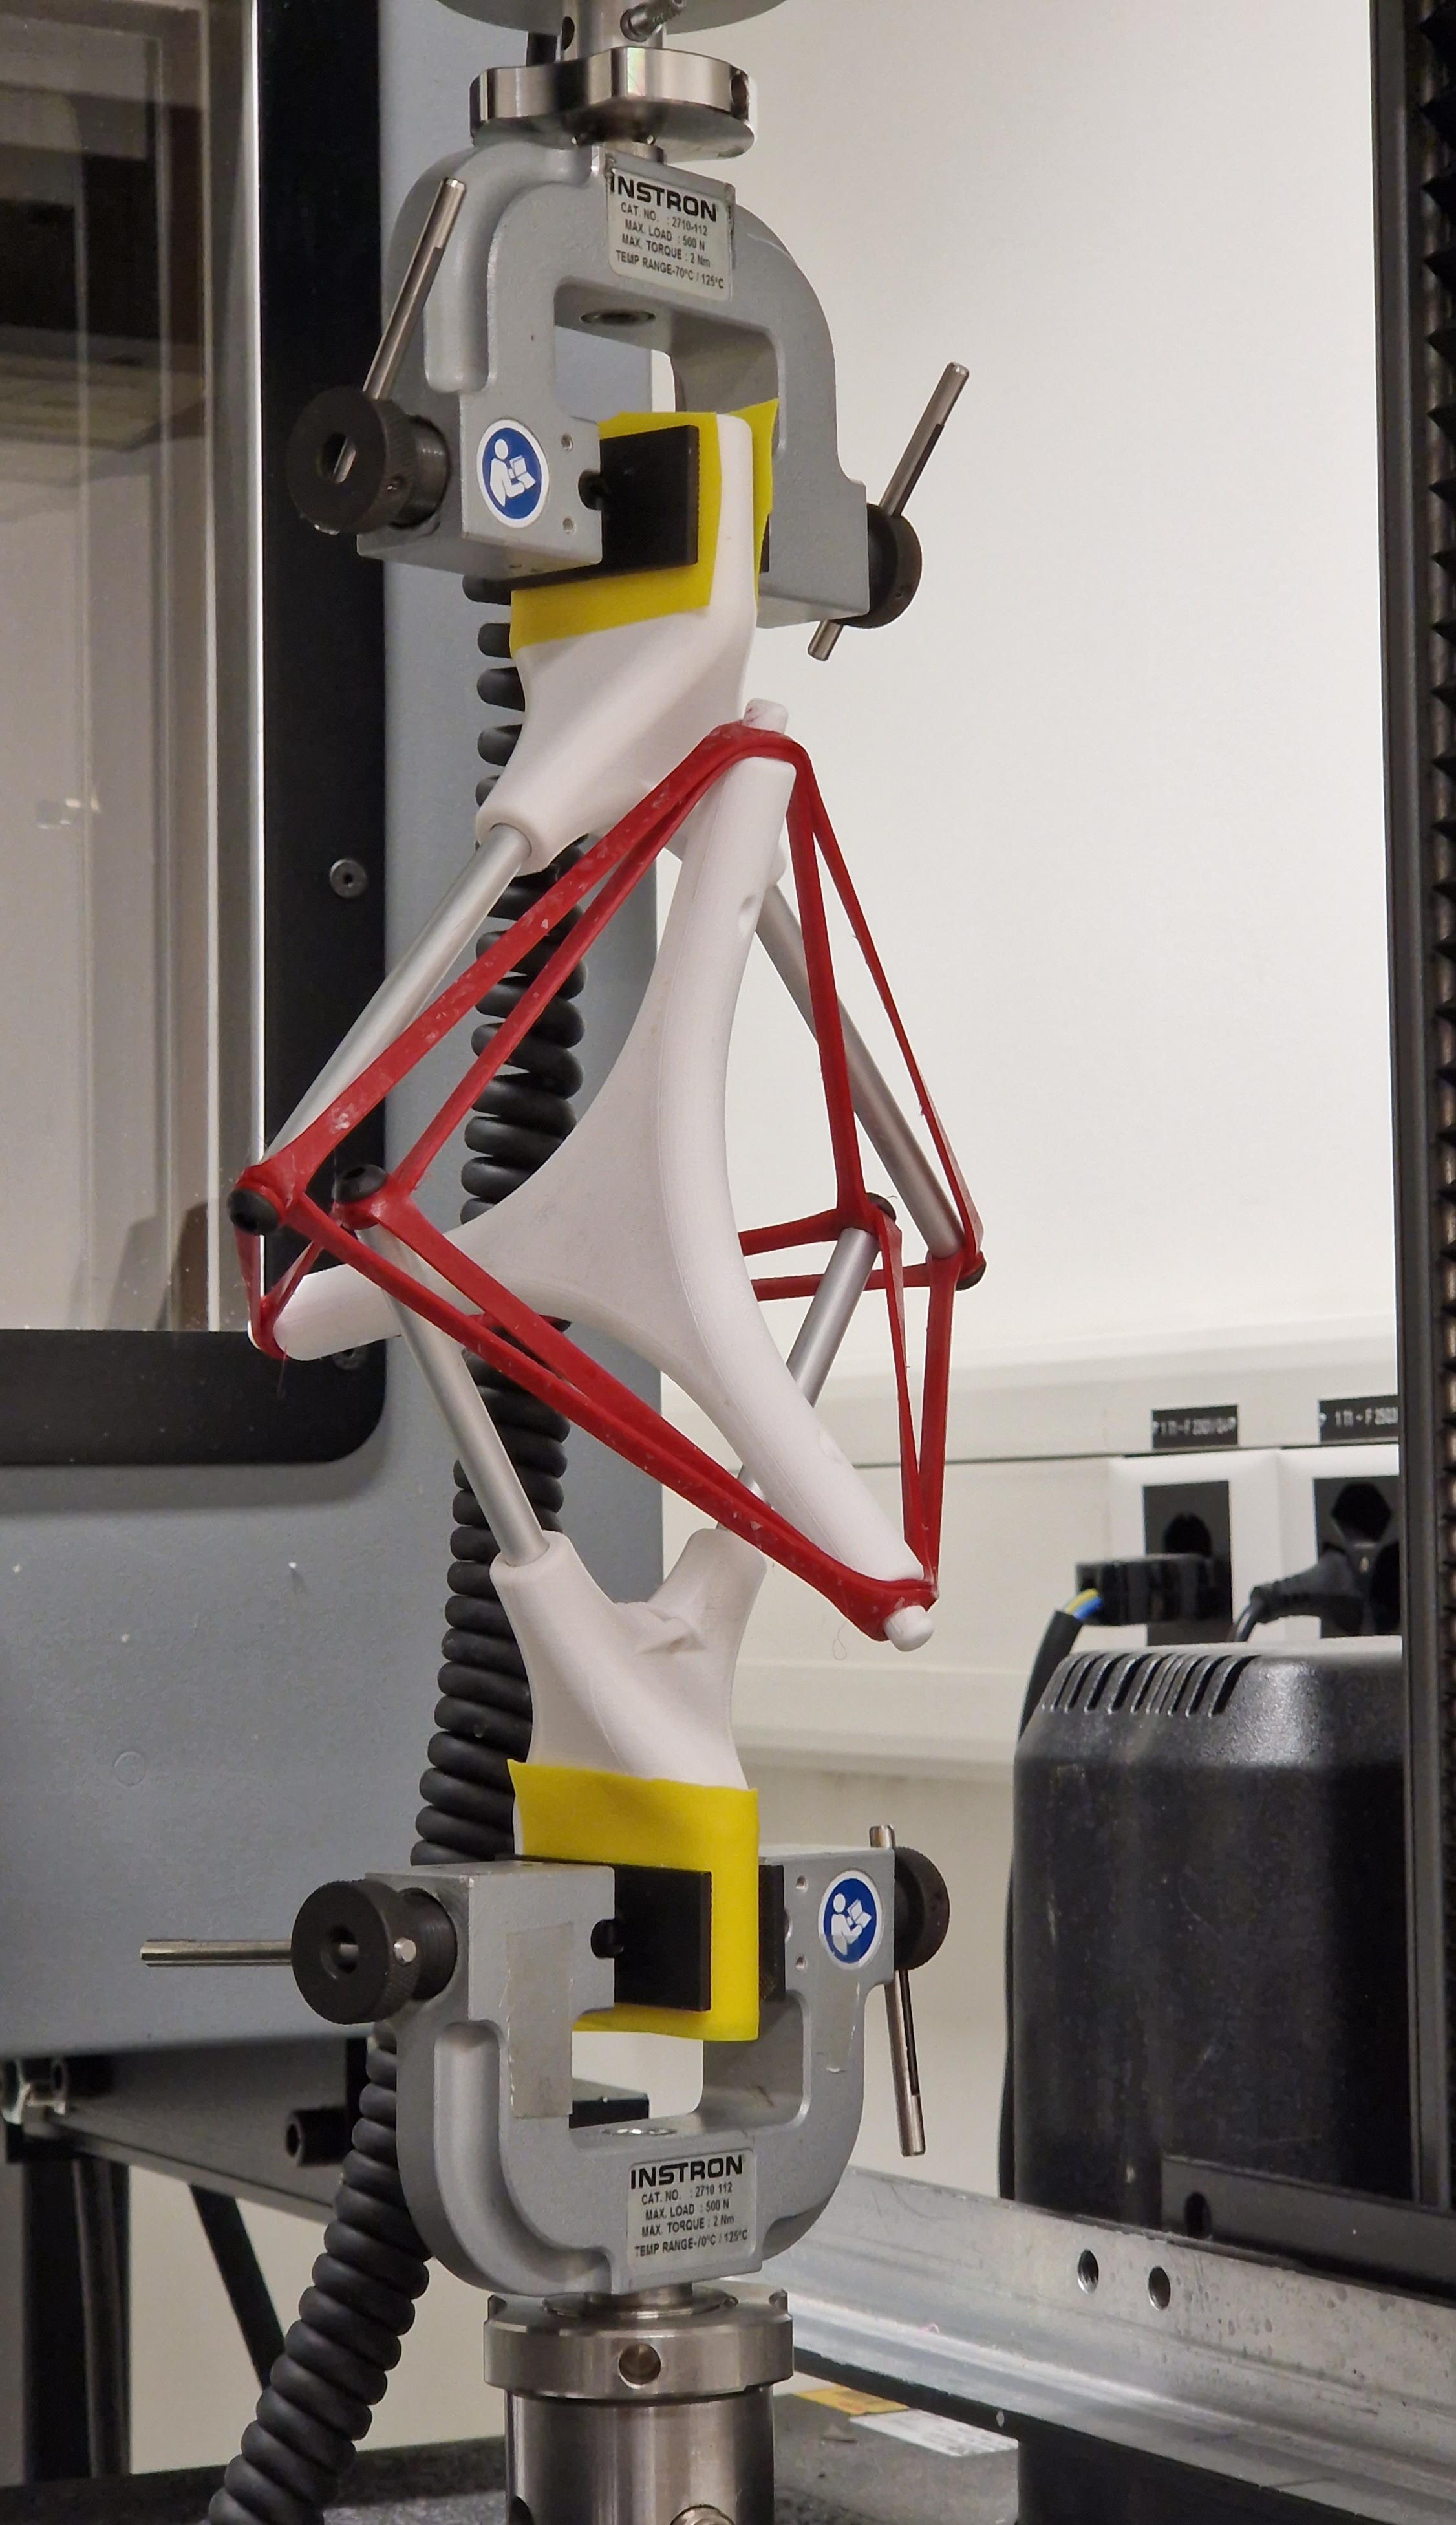}} \quad
\subfloat[Schema representing the test]
{\label{fig:test_compression_schema}%
\includegraphics[width=.35\columnwidth]{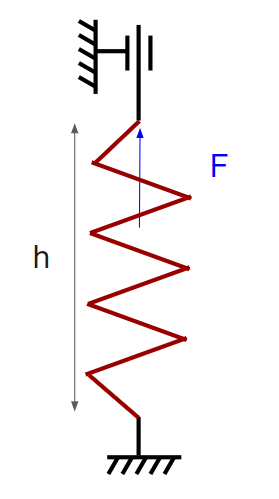}} \quad
\caption{Photo and schema of the test realized on the joint to measure its passive resistance to compression}
\label{fig:test_passive_compression_pictures}
\end{figure}

In this experiment, the two extremities of the joint are clamped to the two sides of the tensile test machine and the angle is set to keep an angle of 180°, as shown on figure \ref{fig:test_compression}. In this disposition, the joint act like a linear spring, as it can not rotate. The machine will then compress the joint by decreasing the value of h with a constant speed of $0.5mm/s$ (until the rigid parts of the joint enter in contact), while measuring the reaction force produced by the joint. This test has been repeated for each of the four sets of joints, and the results are compiled in Figure: \ref{fig:test_passive_compression}. 

\begin{figure}[!h]
\centering 
\includegraphics[width=.8\columnwidth]{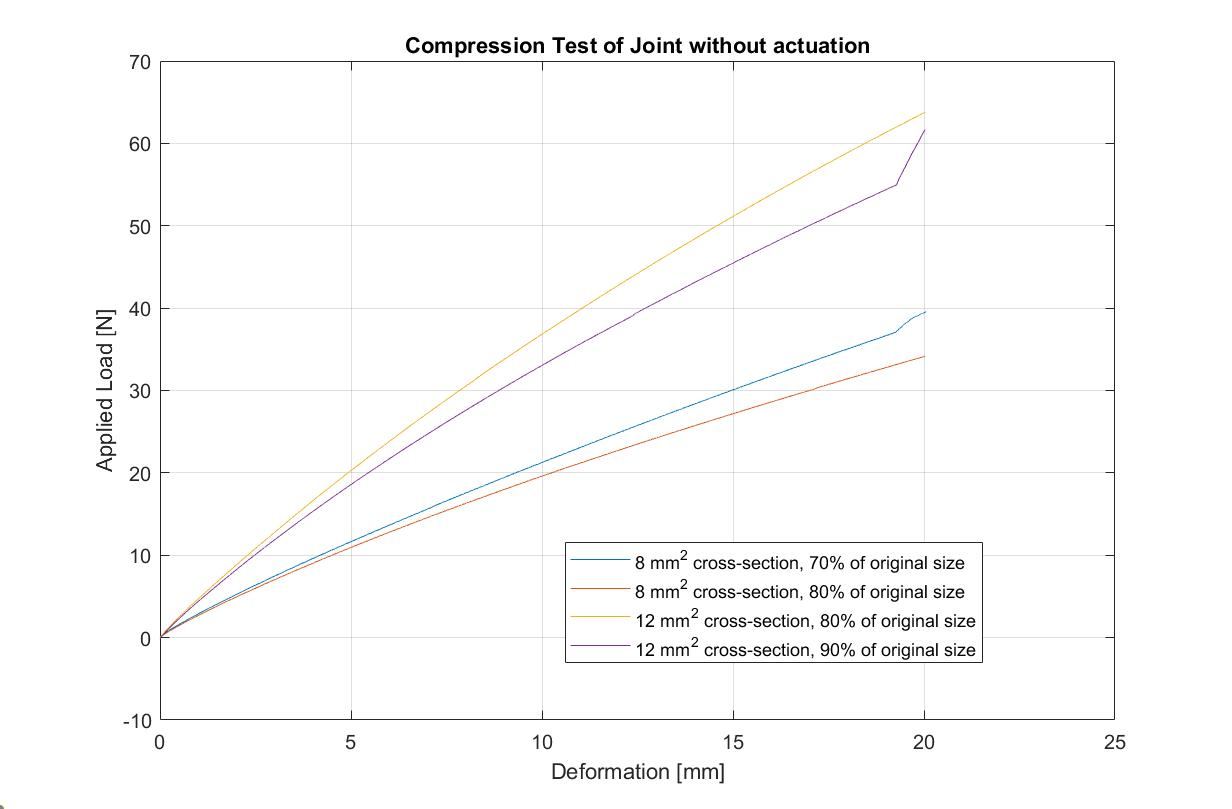} 
\caption{Plot of the measured passive resistance to coaxial compression of the joint without actuation and for different sizing of tendons}
\label{fig:test_passive_compression} 
\end{figure}

This graph shows that increasing both cross-sectional area and pretension level improve the resistance to coaxial loading of the joint. This resistance seems to increase linearly to deformation. It also appears that the sets with a larger cross-section ($12mm^2$) generally oppose more resistance to deformation, due to their improved stiffness.

%It is noticeable that for the four tested sets, those with a cross-section of $12mm^2$ lead to an improved resistance to compression (up to 50\% higher) compared to the sets with a cross-section of $8mm^2$. Then, it is also noticeable that increasing the level of pre-tensioning also increases this resistance but on a smaller scale (up to 10\% increase of a 10\% increase of the pre-tension level). Increasing the cross-section area thus appears to be a better option to improve this resistance.

%The joint's resistance to compression is an important parameter in this tensegrity joint design, as it is essential to keep the two centers of rotation of the Y-Y-Y joint aligned. Indeed, when the joint is deforming in other direction than around its rotation axis, those two rotation axis misalign.  this can lead to difficulties in controlling the joint. It is thus important to keep this value relatively high. On the other hand, as this resistance to compression is a good representation of the overall resistance to deformation of the joint in all non-actuated dimensions, the overall compliance of the joint directly depends on it. In the context of this project, a higher resistance to compression is preferable in order to facilitate the controlling of the joint.

\subsection{Discussion}

In the context of traditional legged robotics, rotational joints are generally supposed to oppose the least possible resistance to rotation. As the developed joint depends on the elastic deformation of the tendons to allow rotation, it opposes a certain degree of resistance to rotation (up to $\SI{2.2}Nm$ for the 80\% $12mm^2$ variant). Nevertheless, the experiments showed that this number can drop to $\SI{1.4}Nm$ by decreasing the degree of pretension to 90\% and can probably drop further more by optimizing these parameters. This behavior could also be considered beneficial if the robot needs to remain stable at a certain position when not actuated (turned off) but this feature will not be considered in this paper.

The joint's resistance to compression is an important parameter in this tensegrity joint design, as it is essential to keep the two centers of rotation of the joint aligned. Indeed, when the joint is deforming in other direction than around its rotation axis, those two rotation axis misalign. This can lead to control difficulties. It is thus important to keep this value relatively high. On the other hand, as this resistance to compression is a good representation of the overall resistance to deformation of the joint in all non-actuated dimensions, the overall compliance of the joint directly depends on it. Certain applications might require high joint compliance. In the context of this project, a higher resistance to compression is preferable in order to facilitate the controlling of the joint.

These experiments indicated that the 90\% $12mm^2$ variant offers the lowest resistance to rotation while keeping a relatively high resistance to coaxial loading. It will thus be used for the other experiments.
